# Supplementary material for: Pinning and gyration dynamics of magnetic vortices revealed by correlative Lorentz and bright-field imaging
Source: arXiv:2107.10208 ancillary file (2021-07-21)
Supplement: Supplementary file 1 [file Supplementary_Information.pdf]

# Supplementary Note1: Electrical setup and corrections

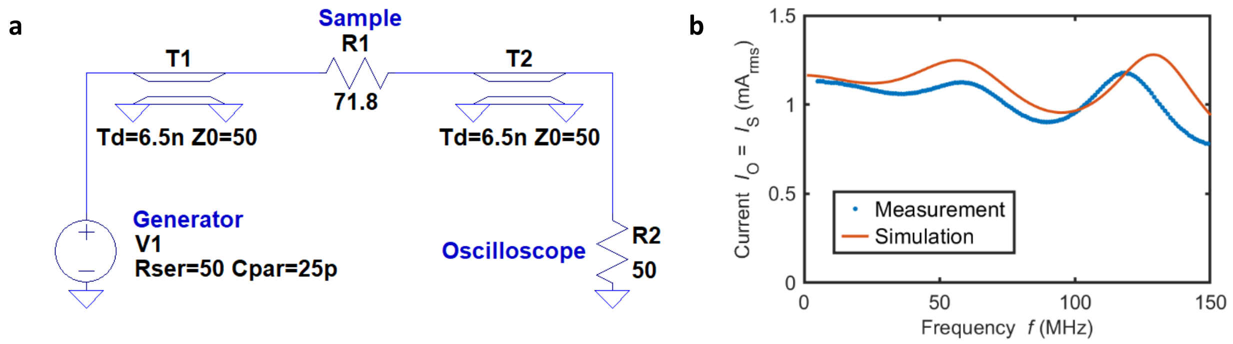


Supplementary Figure 1: Electrical setup for the time-resolved measurement. (a) Circuit diagram of the electrical setup consisting of a voltage source (V1 $= V_G$) with a series resistance (Rser) and a parallel capacitance (Cpar), two 50 Ω transmission lines with a length of 6.5 ns (T1, T2) as well as a resistor for the sample (R1 $= R_S$) and the oscilloscope (R2). (b) Current $I_S$ flowing through the sample as a function of excitation frequency $f_{ex}$ at a generator voltage $V_G = 100\ \mathrm{mV_{rms}}$. The blue dots represent data obtained for sample **A**, whereas the red line stems from a frequency-domain simulation of the circuit in (a).

A circuit diagram of the electrical setup we use in the time-resolved measurement is given in Supplementary Figure 1a. In the experiment, the sample is connected in series between a Keysight 81160 generator (350 MHz bandwidth) and a Tektronix DPO71604C oscilloscope (16 GHz bandwidth) via two identical coaxial cables to both sides of sample.

## Determining the sample resistance

At low frequencies (DC to kHz-range) this setup can be viewed as a voltage source with three resistors in series, i.e. the 50 Ω resistors of the generator and the oscilloscope and the sample itself. Knowing the voltage $V_O$ at the oscilloscope and the generator output voltage $V_G$, we can calculate the sample resistance via:

$$R_S = 2\ \cdot 50\ \Omega \cdot \frac{V_G - V_O}{V_O}.$$

Please note, that here $V_G$ refers to the voltage that is set at the front panel of the generator. This corresponds to half the voltage that is applied across the whole circuit, since usually half of the total voltage is dropped at the generator's internal termination and the other half across a matched 50 Ω load. We measure the exemplary value of $R_{S,A} = 71.8\ \Omega$ in Suppl. Fig. 1a on sample **A** at $V_G = 100\ \mathrm{mV_{rms}}$ and $f_{ex} = 5\ \mathrm{kHz}$ .

## Correcting for standing waves

At higher frequencies, a small impedance mismatch at the output of the generator and a larger mismatch at the sample result in a standing wave between these components. If we were to operate the generator at a constant output voltage, the current $I_S$ passing through the sample would vary with the excitation frequency $f_{ex}$. Since the high-bandwidth input of the oscilloscope shows virtually no reflections in the

spectral range used here, there are no standing waves between the sample and the oscilloscope and therefore $I_S$ is equal to current $I_O$ into the oscilloscope ($I_S = I_O$).

For the time-resolved measurements we generate a look-up table that adapts the generator output voltage $V_G$ such that $I_O$ - and consequently $I_S$ - is kept constant, while sweeping the frequency. To set up this table, we measure $I_O = 50\,\Omega \cdot V_O$ as a function of frequency, where $V_O$ is the voltage measured at the oscilloscope. Supplementary Figure 1b presents an example of such a measurement. The data was recorded on sample **A** at $V_G = 100\ \mathrm{mV_{rms}}$.

Simulating the circuit in Supp. Fig. 1a using LTSpice®[1] XVII reproduces the data obtained from the measurement quite well. The only free parameter in the model is the parasitic capacitance of the generator output. The lengths of the cables were measured using time-domain reflectometry. The good agreement of measurement and simulation show that our assumptions on the circuit are justified.

## Supplementary Note 2: Annealing and Joule Heating

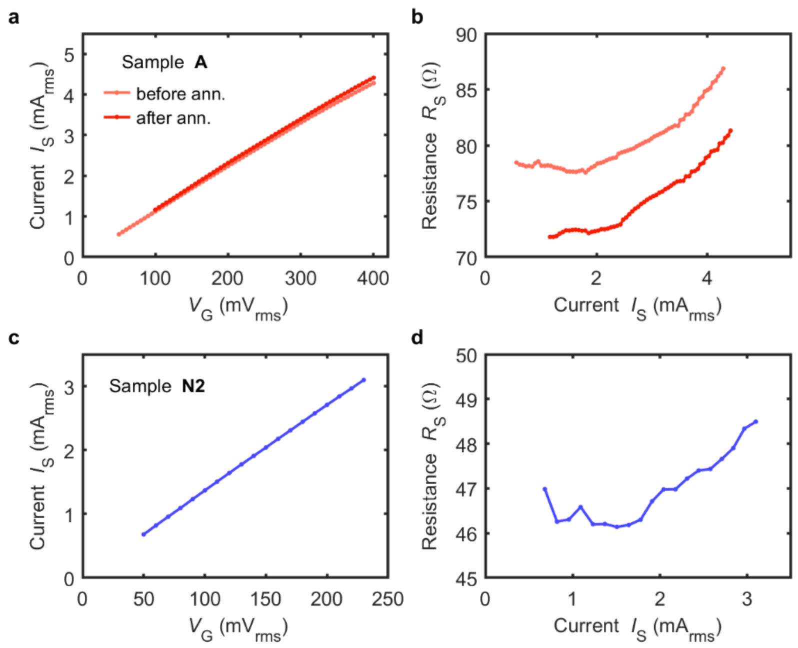


Supplementary Figure 2: Sample current $I_S$ as a function of the generator output voltage $V_G$ and resulting sample resistance $R_S$ for annealed sample **A** (a,b) and non-annealed sample **N2** (c,d). The resistance of sample **A** decreases after annealing, indicating an increase in grain size. For sample **N2** we take special care not to exceed a current threshold that would alter the resistance.

The time-resolved trajectories presented in the main text were measured at two types of samples. Sample **A** has been annealed at a high current ($V_G = 450\ \mathrm{mV_{rms}}$) for $30\ \mathrm{min}$ prior to the time-resolved

[1] LTSpice® is a registered trademark of ANALOG DEVICES, Inc. .

measurement, while great care has been taken to prevent any amount of annealing for sample **N2** ("non-annealed").

Before and after the annealing we measure the sample current $I_\mathrm{S}$ at various generator voltages $V_\mathrm{G}$. From this data we derive the sample resistance $R_\mathrm{S}$ using the equation given in Supplementary Note 1. The results of this measurements are plotted in Supplementary Fig. 2 a,b and show to distinct features: Most prominent is a substantial reduction in sample resistance as a direct consequence of the annealing process. Secondly, we can identify a transient increase in sample resistance at high currents, which is due to a temperature rise caused by Joule heating.

In case of the non-annealed sample, we only allowed for currents below a threshold of non-reversible resistance changes, making sure its grain structure was not altered.

The time-resolved measurements have been conducted at currents of $I_\mathrm{S} = 4.9\,\mathrm{mA_{rms}}$ and $I_\mathrm{S} = 2.2\,\mathrm{mA_{rms}}$ for sample **A** and sample **N2**, respectively. Because of the heat generated by these currents, we found a respective drop in the saturation magnetization of 30% and 10% with respect to room-temperature value of about $440\,\mathrm{A/m}$. These values were derived from Lorentz micrographs of the heated and unheated samples in comparison to simulated Lorentz images. The simulated images were generated using a combination of micro-magnetic[1] and Lorentz image simulation[2]. Details on the technique are discussed in the Supplementary of Ref. 3.

## Additional Supplementary Figures

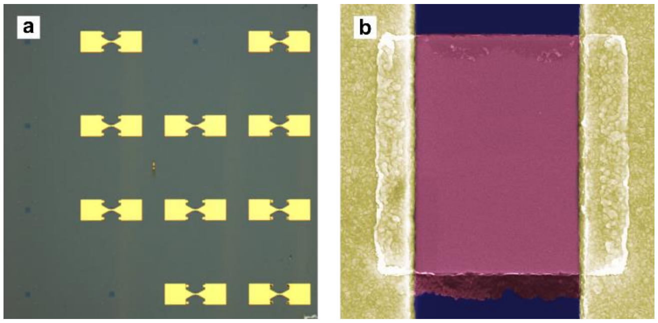


Supplementary Figure 4: Sample system: (a) Light microscope image of a sample frame with 16 silicon nitride windows (small blue squares). The bow-tie-like structures comprise the wire-bonding pads on their sides and taper towards their center, contacting the magnetic microstructure. (b) False-colored scanning electron micrograph sample **A**. The permalloy square (red) is contacted with cold contacts (yellow) and rests on an amorphous silicon nitride membrane. The micrograph was acquired with an acceleration voltage of 10kV using an in-lens detector.

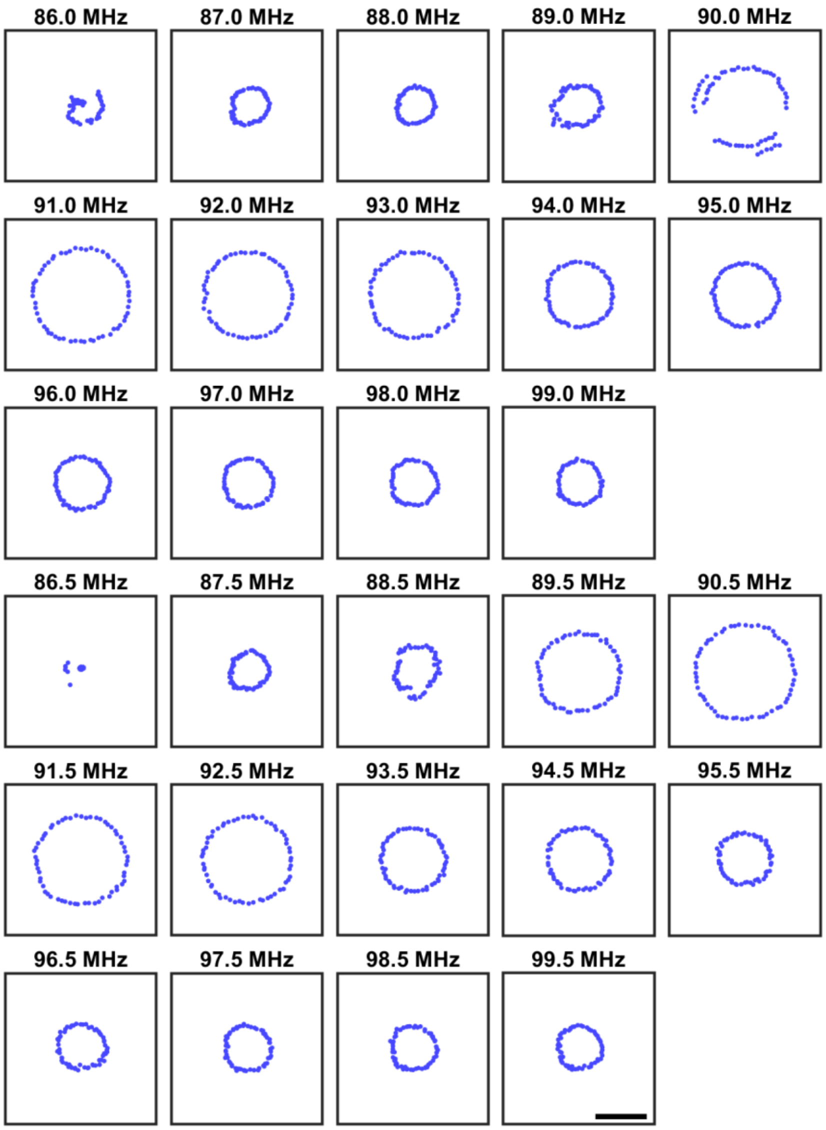


Supplementary Figure 5: Vortex core orbits of non-annealed sample **N2** measured using time-resolved Lorentz microscopy sorted in measurement order (scalebar: 200 nm). For trajectories (e.g., at 90 MHz) appear to be bistable.

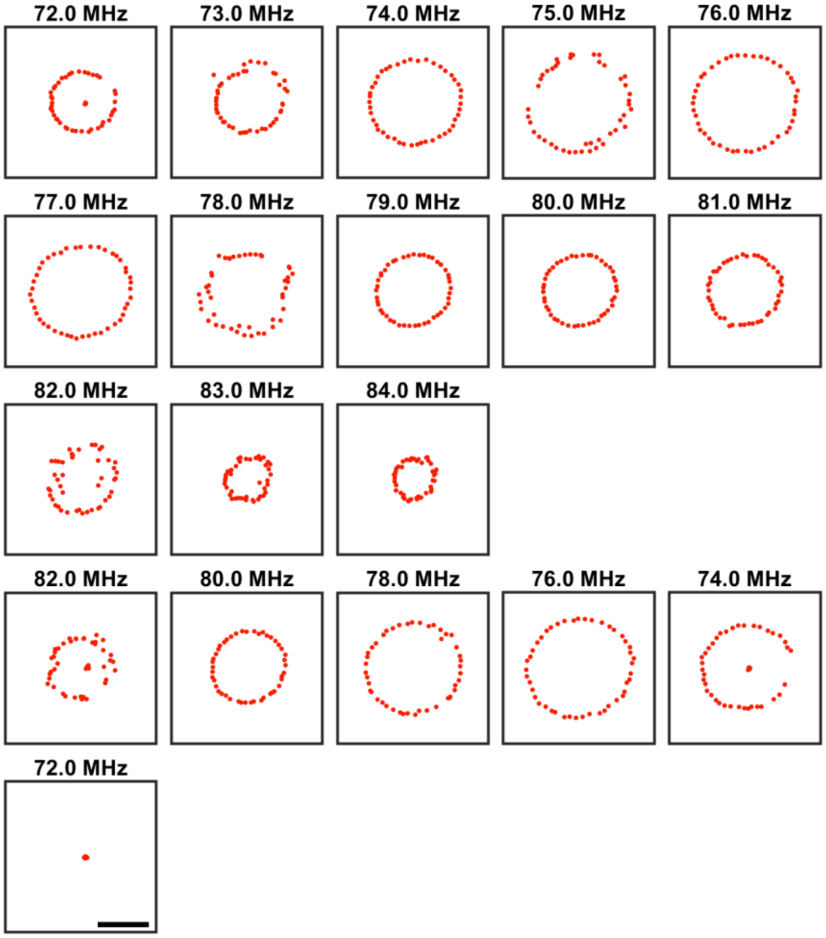


Supplementary Figure 6: Vortex core orbits of non-annealed sample **A** measured using time-resolved Lorentz microscopy sorted in measurement order (scalebar: 200nm). The number of bistable trajectories is higher than for sample **N2** (see Supp. Fig. 5).

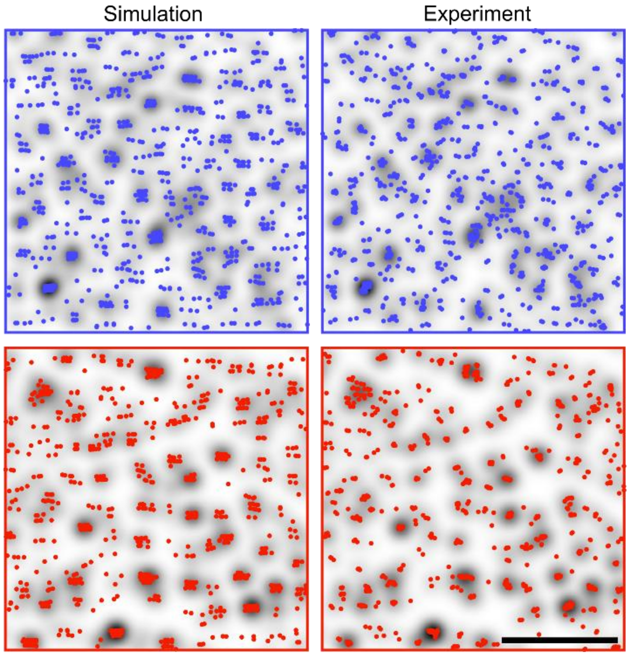


Supplementary Figure 7: Comparison between simulated and experimental TRaPS data for samples **N2** (blue) and **A** (red). The simulated data as well as the underlaid potential (grey) shown here, correspond to the choice of $E_{\mathrm{pin}}$ and $\sigma_{\mathrm{pin}}$ which minimizes the median radial deviation for the respective sample (scalebar: 200nm).

## Supplementary References


1. Vansteenkiste, A. *et al.* The design and verification of MuMax3. *AIP Adv.* **4**, 137133 (2014).

2. De Graef, M. 2. Lorentz microscopy: Theoretical basis and image simulations. in *Magnetic Imaging and its Application to Materials. Experimental Methods in the Physical Sciences* (eds. De Graef, M. & Zhu, Y.) **36**, 27–67 (Academic Press, 2001).

3. Möller, M., Gaida, J. H., Schäfer, S. & Ropers, C. Few-nm tracking of current-driven magnetic vortex orbits using ultrafast Lorentz microscopy. *Commun. Phys.* **3**, 36 (2020).
